# Supplementary material for: Low-Resource Adaptation of Neural NLP Models
Source: arXiv:2011.04372 source file (2020-11-09)
Supplement: Supplementary file 1 [file appendixA.tex]

\chapter{The First Appendix}
\label{sec:first-app}

\section{First Section}

\section{Second Section}
