# Supplementary material for: Low-Resource Adaptation of Neural NLP Models
Source: arXiv:2011.04372 source file (2020-11-09)
Supplement: Supplementary file 2 [file appendixB.tex]

\chapter{Source Code}
\label{sec:source}
\section{Implementation}
The \texttt{phduio} class is implemented in the following way:
%\lstinputlisting[language = {[LaTeX]{TeX}}]{phduio.cls}
